# Supplementary material for: Point Cloud in the Air
Source: arXiv:2401.00658 source file (2024-01-01)
Supplement: Supplementary file 1 [file AppendixA.tex]

This appendix proves that the estimator in \eqref{eq:LMMSEEstimator} is an LMMSE estimator, and derives its MSE.

Given the samples in \eqref{eq:III1}, an LMMSE estimator estimates the sequence $\bm{s}_+\in\mathcal{C}^L$ symbol-by-symbol by
$\widehat{s}_+[i] = \lambda r[i]+c$,
where the constants $\lambda,c\in\mathbb{C}$ are chosen so that the MSE $\frac{1}{L}\sum_{i=1}^L \left|\widehat{s}_+[i]-s_+[i]\right|^2$ is minimized.

First, the MSE of a linear estimator is given by
\small
\begin{eqnarray}\label{eq:III2}
\hspace{-0.5cm}&& \text{MSE}=\frac{1}{L}\sum_{i=1}^L \left|\sum_{m=1}^M (\lambda h_m-1)s_m[i]+c+\lambda z[i]\right|^2 \nonumber\\
\hspace{-0.5cm}&& = \frac{1}{L}\sum_{i=1}^L \left|\sum_{m=1}^M (\lambda h_m\!-\!1)s_m[i]\right|^2 \!\!+ c\frac{1}{L}\sum_{i=1}^L\left[\sum_{m=1}^M (\lambda h_m\!-\!1)s_m[i]\right]^* \nonumber\\
\hspace{-0.5cm}&& \qquad +~ c^*\frac{1}{L}\sum_{i=1}^L\left[\sum_{m=1}^M (\lambda h_m\!-\!1)s_m[i]\right] + |\lambda|^2\frac{N_0}{T} + |c|^2 \nonumber\\
\hspace{-0.5cm}&& = (\lambda\bm{h\!-\!1})^H\frac{1}{L}\sum_{i=1}^L\!\bm{s^*[i]}\bm{s[i]}^\top\!\!(\lambda\bm{h\!-\!1})\!+\!c(\lambda\bm{h\!-\!1})^H\frac{1}{L}\!\sum_{i=1}^L\!\bm{s^*[i]} \nonumber\\
\hspace{-0.5cm}&& \qquad +~ c^*(\lambda\bm{h-1})^\top\frac{1}{L}\sum_{i=1}^L\bm{s[i]} + |\lambda|^2\frac{N_0}{T} + |c|^2 \nonumber\\
\hspace{-0.5cm}&& = (\lambda\bm{h\!-\!1})^H \bm{V}(\lambda\bm{h\!-\!1})\!+\!c(\lambda\bm{h\!-\!1})^H \bm{\widehat{\mu}}^* + c^*(\lambda\bm{h-1})^\top\bm{\widehat{\mu}} \nonumber\\
\hspace{-0.5cm}&& \qquad +~ |\lambda|^2\frac{N_0}{T} + |c|^2,
\end{eqnarray}
\normalsize
where $\bm{V}$ is as defined in \eqref{eq:V} and $\bm{\widehat{\mu}}$ as in \eqref{eq:mu}. As can be seen, MSE is a quadratic function of both $\lambda$ and $c$. The optimal $\lambda$ and $c$ that minimize the MSE can be obtained by setting:
\begin{eqnarray}
\label{eq:partial1}
\hspace{-1cm}&& \frac{\partial \text{MSE}}{\partial \lambda} = \lambda^*\bm{h}^H\bm{Vh} - \bm{1}^\top\bm{Vh} + c^*\bm{h}^\top\bm{\widehat{\mu}} + \lambda^*\frac{N_0}{T}=0, \\
\label{eq:partial2}
\hspace{-1cm}&& \frac{\partial \text{MSE}}{\partial c} = (\lambda\bm{h-1})^H \bm{\widehat{\mu}}^* + c^* = 0.
\end{eqnarray}

Substituting \eqref{eq:partial2} into \eqref{eq:partial1} yields
\begin{eqnarray*}
\lambda = \frac{\bm{h}^H\left(\bm{V-\bm{\widehat{\mu}}^*\bm{\widehat{\mu}}^\top}\right)\bm{1}}{\bm{h}^H\left(\bm{V-\bm{\widehat{\mu}}^*\bm{\widehat{\mu}}^\top}\right)\bm{h}+\frac{N_0}{T}}.
\end{eqnarray*}

To simplify $\lambda$, let us further define $\bm{D}=\bm{V-\bm{\widehat{\mu}}^*\bm{\widehat{\mu}}^\top}$
and we finally have
\begin{eqnarray*}
\lambda = \frac{\bm{h}^H\bm{D}\bm{1}}{\bm{h}^H\bm{D}\bm{h}+\frac{N_0}{T}},~~c=\left(\bm{1}\!-\!\frac{\bm{h}^H\bm{D1}}{\bm{h}^H\bm{Dh}+\frac{N_0}{T}}\bm{h}\right)^\top \!\!\bm{\widehat{\mu}}.
\end{eqnarray*}
Thus, \eqref{eq:LMMSEEstimator} is the LMMSE estimator that minimizes the MSE. Notice that this is an unbiased estimator since
\begin{equation*}
\frac{1}{L}\sum_{i=1}^L(\widehat{s}_+[i]\!-\!{s}_+[i])= \lambda\bm{h}^\top\bm{\widehat{\mu}} \!+\! (\bm{1}\!-\!\lambda\bm{h})^\top\bm{\widehat{\mu}}\!-\!\bm{1}^\top\bm{\widehat{\mu}}=0.
\end{equation*}

Substituting $\lambda$ and $c$ back into \eqref{eq:III2} yields
\begin{eqnarray*}
\text{MSE} &&\hspace{-0.5cm}= (\lambda\bm{h\!-\!1})^H \bm{V}(\lambda\bm{h\!-\!1})\!-\!(\lambda\bm{h\!-\!1})^\top\bm{\widehat{\mu}}\bm{\widehat{\mu}}^H (\lambda\bm{h\!-\!1})^*   \\
&&\hspace{-1.5cm} \qquad - (\lambda\bm{h\!-\!1})^H\bm{\widehat{\mu}}^*\bm{\widehat{\mu}}^\top (\lambda\bm{h\!-\!1}) + |\lambda|^2\frac{N_0}{T} + |(\lambda\bm{h\!-\!1})^\top\bm{\widehat{\mu}}|^2 \\
&&\hspace{-0.5cm}= (\lambda\bm{h\!-\!1})^H \bm{D}(\lambda\bm{h\!-\!1}) + |\lambda|^2\frac{N_0}{T} \\
&&\hspace{-0.5cm}= \bm{1}^\top\bm{D1}-\frac{\left|\bm{h}^H\bm{D1}\right|^2}{\bm{h}^H\bm{Dh}+\frac{N_0}{T}}.
\end{eqnarray*}

We next compare $\text{MSE}_\text{LMMSE}$ with $\text{MSE}_\text{ML}$. From \eqref{eq:MSENaiveh} and \eqref{eq:MSELMMSEh}, we have
\begin{eqnarray}\label{eq:III3}
\hspace{-0.5cm}&&\text{MSE}_\text{ML} - \text{MSE}_\text{LMMSE} \\
\hspace{-0.5cm}&&= (\bm{h\!-\!1})^H\bm{V}(\bm{h\!-\!1})\!+\!\frac{N_0}{T} \!-\! \left(\bm{1}^\top\bm{D1}\!-\!\frac{\left|\bm{h}^H\bm{D1}\right|^2}{\bm{h}^H\bm{Dh}\!+\!\frac{N_0}{T}} \right). \nonumber
\end{eqnarray}

Multiplying both sides of \eqref{eq:III3} by $\bm{h}^H\bm{Dh}+\frac{N_0}{T}$ and defining
\begin{eqnarray}\label{eq:III4}
q\left(\frac{N_0}{T}\right) \triangleq&&\hspace{-0.55cm} \left(\text{MSE}_\text{ML} - \text{MSE}_\text{LMMSE} \right) \left(\bm{h}^H\bm{Vh}+\frac{N_0}{T} \right) \nonumber\\
=&&\hspace{-0.55cm} \Big(\bm{h}^H\bm{Dh}+\frac{N_0}{T} \Big) \Big(\bm{h}^H\bm{Vh}-\bm{1}^\top\bm{Vh}-\bm{h}^H\bm{V1} \nonumber\\
&&\hspace{-0.5cm} +\bm{1}^\top\bm{V1}-\bm{1}^\top\bm{D1}+\frac{N_0}{T} \Big) + |\bm{1}^\top\bm{Dh}|^2.
\end{eqnarray}
Since $\bm{D}$ is positive definite, we have $\bm{h}^H\bm{Dh}+\frac{N_0}{T}>0$. To prove $\text{MSE}_\text{LMMSE}\leq \text{MSE}_\text{ML}$, we only need to prove the minimum value of $q\left(\frac{N_0}{T}\right)$ is nonnegative.

From \eqref{eq:III4}, we know that $q(N_0/T)$ is a quadratic function of $N_0/T$. Then, $N_0/T$ that minimizes $q(N_0/T)$ can be obtained by setting:
\begin{eqnarray*}
\hspace{-0.5cm}&& \frac{\partial q(N_0/T)}{\partial (N_0/T)} = 2\frac{N_0}{T} + \bm{h}^H\bm{Dh} + \bm{h}^H\bm{Vh} - \bm{1}^\top\bm{Vh} - \bm{h}^H\bm{V1} \\
\hspace{-0.5cm}&& \hspace{2cm}  +~ \bm{1}^\top\bm{V1} - \bm{1}^\top\bm{D1} =0.
\end{eqnarray*}

Since the noise variance cannot be negative, we have
\begin{eqnarray*}
\frac{N_0}{T} =&&\hspace{-0.55cm} \max\Big(0,\frac{1}{2}\big[\bm{1}^\top\bm{D1} - (\bm{h}^H\bm{Dh} + \bm{h}^H\bm{Vh} - \bm{1}^\top\bm{Vh} \\
&&\hspace{-0.55cm} - \bm{h}^H\bm{V1} + \bm{1}^\top\bm{V1}) \big]\Big).
\end{eqnarray*}

1) When $\frac{1}{2}\big[\bm{1}^\top\bm{D1} - (\bm{h}^H\bm{Dh} + \bm{h}^H\bm{Vh} - \bm{1}^\top\bm{Vh} - \bm{h}^H\bm{V1} + \bm{1}^\top\bm{V1}) \big] \leq 0$, we have $N_0/T = 0$ and
\begin{eqnarray*}
\hspace{-0.65cm}&& q\left(\frac{N_0}{T}\right)\geq q(0)= \bm{h}^H\bm{Dh}(\bm{h}^H\bm{Vh}-\bm{1}^\top\bm{Vh}-\bm{h}^H\bm{V1} \\
\hspace{-0.65cm}&& \qquad\qquad +~ \bm{1}^\top\bm{V1}) - \bm{h}^H\bm{Dh}\bm{1}^\top\bm{D1}+|\bm{1}^\top\bm{Dh}|^2
\end{eqnarray*}

Let us define $\bm{E}\triangleq\bm{V-D}=\bm{\widehat{\mu}}^*\bm{\widehat{\mu}}^\top$, then
\begin{eqnarray*}
\hspace{-0.65cm}&& q(0)\!=\! \bm{h}^H\!\bm{Dh}(\bm{h}^H\bm{Vh}\!-\!\bm{1}^\top\!\bm{Vh}\!-\!\bm{h}^H\!\bm{V1}\!+\!\bm{1}^\top\!\bm{E1})\!+\!|\bm{1}^\top\!\bm{Dh}|^2 \\
\hspace{-0.65cm}&& = \bm{h}^H\bm{Dh}(\bm{h}^H\bm{Dh} \!-\! \bm{1}^\top\bm{Dh} \!-\! \bm{h}^H\bm{D1}) + \bm{h}^H\bm{Dh}(\bm{h}^H\bm{Eh} \\
\hspace{-0.65cm}&&  \qquad -~ \bm{1}^\top\bm{Eh} \!-\! \bm{h}^H\bm{E1} \!+\! \bm{1}^\top\bm{E1})+|\bm{1}^\top\bm{Dh}|^2 \\
\hspace{-0.65cm}&& = (\bm{h\!-\!1})^H\bm{Dh}\bm{h}^H\bm{D}(\bm{h\!-\!1}) \!+\! \bm{h}^H\bm{Dh}(\bm{h\!-\!1})^H\bm{E}(\bm{h\!-\!1}) \\
\hspace{-0.65cm}&& = |(\bm{h\!-\!1})^H\bm{Dh}|^2 +\bm{h}^H\bm{Dh}|(\bm{h\!-\!1})^\top\bm{\widehat{\mu}}|^2 \geq 0,
\end{eqnarray*}
where the last inequality follows because $\bm{D}$ is positive definite.
Therefore,
\begin{eqnarray*}
\text{MSE}_\text{ML}- \text{MSE}_\text{LMMSE}
\geq \frac{q(0)}{\bm{h}^H\bm{Dh}}\geq 0.
\end{eqnarray*}
This formula matches our intuition: when the noise variance $N_0/T=0$ and the channel precoding is perfect, i.e., $\bm{h=1}$, we have $q(0)=0$. The ML and the LMMSE estimators are the same in this case as $\lambda=1$ and $c=0$.

% x1 = \bm{h}^H\bm{Vh}
% x2 = \bm{1}^\top\bm{Vh}
% x2* = \bm{h}^H\bm{V1}
% x3 = \bm{1}^\top\bm{V1}

2) When $\frac{1}{2}\big[\bm{1}^\top\bm{D1} - (\bm{h}^H\bm{Dh} + \bm{h}^H\bm{Vh} - \bm{1}^\top\bm{Vh} - \bm{h}^H\bm{V1} + \bm{1}^\top\bm{V1}) \big] > 0$, we have
\begin{eqnarray*}
\hspace{-0.5cm}&& q\left(\frac{N_0}{T}\right)\geq q\Big(\frac{1}{2}\big[\bm{1}^\top\bm{D1} - (\bm{h}^H\bm{Dh} + \bm{h}^H\bm{Vh} - \bm{1}^\top\bm{Vh} \\
\hspace{-0.5cm}&& \qquad\qquad -~ \bm{h}^H\bm{V1} + \bm{1}^\top\bm{V1}) \big]\Big) \\
\hspace{-0.5cm}&& = |\bm{1}^\top\bm{Dh}|^2 -\frac{1}{4}\Big(\bm{1}^\top\bm{Vh}+\bm{h}^H\bm{V1}-\bm{h}^H\bm{Eh}-\bm{1}^\top\bm{E1}  \Big)^2 \\
\hspace{-0.5cm}&& = |\bm{1}^\top\bm{Dh}|^2 -\frac{1}{4}\Big[\bm{1}^\top\bm{Dh}+\bm{h}^H\bm{D1}\!-\!(\bm{h\!-\!1})^H\bm{E}(\bm{h\!-\!1})  \Big]^2 \\
\hspace{-0.5cm}&& = |\bm{1}^\top\bm{Dh}|^2 - \frac{1}{4}\Big[ 2(\bm{1}^\top\bm{Dh})^\mathfrak{r} - |(\bm{h\!-\!1})^\top\bm{\widehat{\mu}}|^2 \Big]^2 \\
\hspace{-0.5cm}&& \overset{(a)}{\geq} |\bm{1}^\top\bm{Dh}|^2 -\left[(\bm{1}^\top\bm{Dh})^\mathfrak{r} \right]^2= \left[(\bm{1}^\top\bm{Dh})^\mathfrak{i} \right]^2 \geq 0
\end{eqnarray*}
where (a) follows from $\frac{1}{2}\big[\bm{1}^\top\bm{D1} - (\bm{h}^H\bm{Dh} + \bm{h}^H\bm{Vh} - \bm{1}^\top\bm{Vh} - \bm{h}^H\bm{V1} + \bm{1}^\top\bm{V1}) \big] > 0$. That is, we have $\bm{1}^\top\bm{Vh}+\bm{h}^H\bm{V1}-\bm{h}^H\bm{Eh}-\bm{1}^\top\bm{E1}\geq 0$, and hence $2(\bm{1}^\top\bm{Dh})^\mathfrak{r} - |(\bm{h\!-\!1})^\top\bm{\widehat{\mu}}|^2>0$.

Overall, we have $\text{MSE}_\text{LMMSE}\leq \text{MSE}_\text{ML}$.
