# Supplementary material for: Point Cloud in the Air
Source: arXiv:2401.00658 source file (2024-01-01)
Supplement: Supplementary file 2 [file AppendixA2.tex]

This appendix proves Theorem \ref{thm:prop7}. 
We first show that the estimator in \eqref{eq:LMMSE_misaligned} is an LMMSE estimator.
Given the signal model in \eqref{eq:samplesMat}, a linear estimator estimates $\bm{s}_+$ by
$\widehat{\bm{s}}_+=\bm{A y+c}$.
The MSE of the linear estimate $\widehat{\bm{s}}_+$ is then given by
\begin{eqnarray}\label{eq:MSE_mislaigned}
\text{MSE}=\frac{1}{L}\mathbb{E}\left[(\bm{Ay+c}-{\bm{s}}_+)^H(\bm{Ay+c}-{\bm{s}}_+)\right].
\end{eqnarray}

The matrix $\bm{A}$ and vector $\bm{c}$ that yield the minimum MSE can then be obtained by setting $\partial\text{MSE}/\partial\bm{A}=0$ and $\partial\text{MSE}/\partial\bm{c}=0$. Thus, we have
\begin{eqnarray*}
\hspace{-0.65cm}&&\frac{\partial\text{MSE}}{\partial\bm{A}}=\mathbb{E}\frac{\partial\text{Tr}[(\bm{Ay+c}-{\bm{s}}_+)(\bm{Ay+c}-{\bm{s}}_+)^H]}{\partial\bm{A}} \\
\hspace{-0.65cm}&&=\!\bm{A}\mathbb{E}[\bm{yy^H}] +\bm{c}\mathbb{E}^H[\bm{y}]-\mathbb{E}[\bm{s_+}\bm{y^H}]\\
\hspace{-0.65cm}&&=\!\! \bm{AG\mathbb{E}[ss^H]G^H\!\!+\!\!A\Sigma_z}\!+\!\bm{c\mathbb{E}^H[s]G^H}\!\!-\!\bm{F\mathbb{E}[ss^H]G^H}\!\!=\!0, \\
\hspace{-0.65cm}&&\frac{\partial\text{MSE}}{\partial\bm{c}}\!=\!\bm{A\mathbb{E}[y]\!+\!c\!-\!\mathbb{E}[s_+]} \!=\! \bm{AG\mathbb{E}[s]}\!+\!\bm{c}\!-\!\bm{F\mathbb{E}[s]}\!=\!0.
\end{eqnarray*}
Given $\widetilde{\bm{\mu}}=\mathbb{E}[\bm{s}]$ and $\bm{\widetilde{D}}=\mathbb{E}[\bm{ss^H}]-\mathbb{E}[\bm{s}]\mathbb{E}^H[\bm{s}]$, we have
\begin{eqnarray*}
\bm{A}
\hspace{-0.2cm}&=&\hspace{-0.2cm} \bm{F\widetilde{D}G^H}(\bm{G\widetilde{D}G^H}+\bm{\Sigma_z})^{-1}, \\
\bm{c}
\hspace{-0.2cm}&=&\hspace{-0.2cm} \bm{F}\widetilde{\bm{\mu}}-\bm{AG}\widetilde{\bm{\mu}}.
\end{eqnarray*}
This gives us the LMMSE estimator in \eqref{eq:LMMSE_misaligned}. The MSE of the LMMSE estimator can be obtained by substituting $\bm{A}$ and $\bm{c}$ into \eqref{eq:MSE_mislaigned}, giving
\begin{eqnarray*}
&&\hspace{-0.5cm} \text{MSE}=\frac{1}{L}\mathbb{E}\left[(\bm{Ay+c}-{\bm{s}}_+)^H(\bm{Ay+c}-{\bm{s}}_+)\right] \\
&&\hspace{-0.5cm} = \frac{1}{L}\mathbb{E}\left\{\left[(\bm{AG\!-\!F})\bm{s\!+\!Az\!+\!c}\right]^H\left[(\bm{AG\!-\!F})\bm{s\!+\!Az\!+\!c}\right]\right\} \\
&&\hspace{-0.5cm} = \frac{1}{L}\mathbb{E}\big[\bm{s}^H(\bm{AG-F})^H(\bm{AG-F})\bm{s}+\bm{c}^H(\bm{AG-F})\bm{s}+\\
&&\hspace{-0.5cm} \qquad\bm{z}^H\bm{A}^H\bm{Az} + \bm{s}^H(\bm{AG-F})^H\bm{c}+\bm{c}^H\bm{c} \big] \\
&&\hspace{-0.5cm} \overset{(a)}{=} \frac{1}{L}\mathbb{E}\big[\bm{s}^H(\bm{AG-F})^H(\bm{AG-F})\bm{s}+\bm{z}^H\bm{A}^H\bm{Az}\\
&&\hspace{-0.5cm}  \qquad- \frac{1}{L}\widetilde{\bm{\mu}}^H(\bm{AG-F})^H(\bm{AG-F})\widetilde{\bm{\mu}} \big]\\
&&\hspace{-0.5cm} =\! \frac{1}{L}\text{Tr}\left\{ (\bm{AG\!\!-\!\!F})(\mathbb{E}[\bm{ss}^H]\!\!-\!\!\widetilde{\bm{\mu}}\widetilde{\bm{\mu}}^H)(\bm{AG\!\!-\!\!F})^H\!+\!\bm{A\Sigma_zA}^H \right\} \\
&&\hspace{-0.5cm}= \frac{1}{L}\text{Tr}\left[(\bm{AG\!-\!F})\widetilde{\bm{D}}(\bm{AG\!-\!F})^H  \!+\! \bm{A\Sigma_zA}^H \right],
\end{eqnarray*}
where (a) follows by substituting $\bm{c}=(\bm{F}-\bm{AG})\widetilde{\bm{\mu}}$.
