# Supplementary material for: Point Cloud in the Air
Source: arXiv:2401.00658 source file (2024-01-01)
Supplement: Supplementary file 3 [file AppendixB.tex]

This appendix proves Theorem \ref{thm:AMP}.
Note that the key of Theorem \ref{thm:AMP} is the first part that the marginal posterior distribution $f(\bm{s[i]} |\allowbreak \bm{y})$ is an $M$-dimensional complex Gaussian distribution. Provided that this argument is right, the rest of Theorem \ref{thm:AMP} holds.
In the following, let us dive deeper into the analog message passing and prove that $f(\bm{s[i]} |\allowbreak \bm{y})$ is an $M$-dimensional complex Gaussian distribution and can be computed by Algorithm \ref{algo:1}.

To begin with, we point out that a multivariate Gaussian distribution can be parameterized by two sets of parameters \cite{gauvain1994maximum,ahrendt2005multivariate,bromiley2003products}: the moment parameter $(\bm{\mu},\bm{\Sigma})$ and the canonical parament $(\bm{\eta},\bm{\Lambda})$. The two sets of parameters can be transformed into one another and they are useful in different circumstances, as detailed below.

{\bf The moment parameters} $(\bm{\mu},\bm{\Sigma})$. For a multivariate real Gaussian random variable $\bm{w}$ of dimension $2M$, its moment parameters are defined as
\begin{eqnarray*}
\bm{\mu} = \mathbb{E}[\bm{w}],~~\bm{\Sigma} = \mathbb{E}\left[(\bm{w-\mu})(\bm{w-\mu})^\top \right].
\end{eqnarray*}
The moment form of the Gaussian distribution is given by
\begin{small}
\begin{eqnarray*}
\mathcal{N}(\bm{w};\bm{\mu},\!\bm{\Sigma})=\frac{1}{(2\pi)^M|\bm{\Sigma}|^{\frac{1}{2}}} \exp \left\{\!-\frac{1}{2}(\bm{w\!-\!\mu})^\top \bm{\Sigma}^\dagger (\bm{w\!-\!\mu})\!\right\}.
\end{eqnarray*}
\end{small}

\begin{lem}[Marginalization of a multivariate Gaussian \cite{ahrendt2005multivariate}]\label{lemma1}
Let $\bm{w}\sim\mathcal{N}(\bm{w};\bm{\mu},\!\bm{\Sigma})$ be a multivariate Gaussian random variable of dimension $2M$ with the moment parameters being $(\bm{\mu},\bm{\Sigma})$. Let us partition $\bm{w}=[\bm{w_1},\bm{w_2}]^\top$ where $\bm{w_1}$, $\bm{w_2}$ are multivariate Gaussians of dimension $\kappa$ and $2M-\kappa$, respectively. The moment parameters can be partitioned accordingly as
\begin{eqnarray*}
\bm{\mu}=\begin{bmatrix}
\bm{\mu_1} \\
\bm{\mu_2}
\end{bmatrix},~~~
\bm{\Sigma}=\begin{bmatrix}
\bm{\Sigma_{11}} & \bm{\Sigma_{12}} \\
\bm{\Sigma_{21}} & \bm{\Sigma_{22}}
\end{bmatrix}.
\end{eqnarray*}
If we marginalize out $\bm{w_2}$ from $\bm{w}$, the marginal $f(\bm{w_1})$ is still a Gaussian distribution, giving
\begin{eqnarray}
f(\bm{w_1})\hspace{-0.2cm}&=&\hspace{-0.2cm}\int_{\bm{w_2}} \mathcal{N}\left(\begin{bmatrix}
\bm{w_1} \\
\bm{w_2}
\end{bmatrix};\begin{bmatrix}
\bm{\mu_1} \\
\bm{\mu_2}
\end{bmatrix},\!\begin{bmatrix}
\bm{\Sigma_{11}} & \bm{\Sigma_{12}} \\
\bm{\Sigma_{21}} & \bm{\Sigma_{22}}
\end{bmatrix}\right) d\bm{w_2} \nonumber\\
\hspace{-0.2cm}&\propto&\hspace{-0.2cm}
\mathcal{N}(\bm{w_1};\bm{\mu_1},\!\bm{\Sigma_{11}}).
\end{eqnarray}
\end{lem}

{\bf The canonical paraments} $(\bm{\eta},\bm{\Lambda})$. For a Gaussian random variable $\bm{w}$ of dimension $2M$, its canonical parameters are defined as
\begin{eqnarray*}
\bm{\eta} = \Sigma^\dagger \bm{\mu},~~~  \bm{\Lambda} = \Sigma^\dagger.
\end{eqnarray*}

The canonical form of the Gaussian distribution is given by
\begin{eqnarray*}
\mathcal{N}(\bm{w};\bm{\eta},\bm{\Lambda})=\exp \left\{-\frac{1}{2}\bm{w}^\top\bm{\Lambda}\bm{w}+\bm{w}^\top\bm{\eta}+\rho   \right\},
\end{eqnarray*}
where $\rho$ is a constant
\begin{eqnarray*}
\rho = -\frac{1}{2}\left(2M\ln 2\pi -\ln |\bm{\Lambda}| + \bm{\eta}^\top \bm{\Lambda}^\dagger \bm{\eta} \right).
\end{eqnarray*}

\begin{lem}[Product of multivariate Gaussians \cite{bromiley2003products}]\label{lemma2}
Let $\{\bm{w_k}: k=1,2,...,K\}$, $\bm{w_k}\sim\mathcal{N}(\bm{w}; \bm{\eta_k}, \bm{\Lambda_k})$ be a set of multivariate real Gaussian random variable of dimension $2M$. Then, the product of them is still a Gaussian with the new canonical parameters being the sum of the canonical parameters of the original $K$ Gaussians.
\begin{eqnarray}
\hspace{-0.5cm}&& \prod_{k=1}^{K}\mathcal{N}(\bm{w_k};\bm{\eta_k},\bm{\Lambda_k}) \propto \mathcal{N}\left(\bm{w};\sum_{k=1}^K\bm{\eta_k},\sum_{k=1}^K\bm{\Lambda_k}\right) \\
\hspace{-0.5cm}&& \propto \exp \left\{-\frac{1}{2}\bm{w}^\top \sum_{k=1}^K \bm{\Lambda_k}\bm{w} +\bm{w}^\top\sum_{k=1}^K\bm{\eta_k} + \sum_{k=1}^K{\rho_k} \right\}. \nonumber
\end{eqnarray}
\end{lem}

Now that the factor graph in Fig.~\ref{fig:5} has a tree structure, we only need to pass the messages from left to right (forward message passing) and then from right to left (backward message passing). Each message needs to be computed only once, after which the exact marginal posterior distribution converges.

{\it \textbf{Forward Message Passing}} -- We first investigate how the messages are passed from left to right in Fig.~\ref{fig:5}. Without loss of generality, we shall focus on message passing from one variable $\bm{W_{k,i}}$ to another variable $\bm{W_{k+1,i}}$ on the right.

Notice that $\bm{W_{k,i}}=\allowbreak \mathcal{V}(y_k[i])=\{\allowbreak s_1[i],...,\allowbreak s_k[i],\allowbreak s_{k+1}[i-1],\allowbreak s_{k+2}[i-1],\allowbreak ...,s_M[i-1]\}$ and $\bm{W_{k+1,i}}=\allowbreak \mathcal{V}(y_{k+1}[i])=\{\allowbreak s_1[i],...,\allowbreak s_k[i],\allowbreak s_{k+1}[i],\allowbreak s_{k+2}[i-1],\allowbreak ...,s_M[i-1]\}$. Thus, the only difference between $\bm{W_{k,i}}$ and $\bm{W_{k+1,i}}$ is the $(k+1)$-th symbol.
We consider each complex random variable $s_k[i]$ as a real random vector with the elements being the real and imaginary parts. Then, each $\bm{W_{k,i}}$ can be viewed as a $2M$-dimensional real random variable. To simplify the notation, we denote the $2M$-dimensional real variates corresponding to $\bm{W_{k,i}}$ and $\bm{W_{k+1,i}}$, respectively, by

\footnotesize
\begin{eqnarray*}
\bm{w_{k,i}} \hspace{-0.3cm}&=&\hspace{-0.3cm}\! \left(\!b^\mathfrak{r}_1,...,b^\mathfrak{r}_k,b^\mathfrak{r}_{k+1},b^\mathfrak{r}_{k+2},...,b^\mathfrak{r}_M,
b^\mathfrak{i}_1,...,b^\mathfrak{i}_k,b^\mathfrak{i}_{k+1},b^\mathfrak{i}_{k+2},...,b^\mathfrak{i}_M \! \right), \\
\bm{w_{k+1,i}} \hspace{-0.3cm}&=&\hspace{-0.3cm}\! \left(\! b^\mathfrak{r}_1,...,b^\mathfrak{r}_k,c^\mathfrak{r}_{k+1},b^\mathfrak{r}_{k+2},...,b^\mathfrak{r}_M,
b^\mathfrak{i}_1,...,b^\mathfrak{i}_k,c^\mathfrak{i}_{k+1},b^\mathfrak{i}_{k+2},...,b^\mathfrak{i}_M \! \right),
\end{eqnarray*}
\normalsize
as shown in Fig.~\ref{fig:6}.

On the left half of Fig.~\ref{fig:6}, there are four edges centered around the equality function ``$=$'' (marked in blue). Due to the equality constraint, these four edges are associated with the same high-dimensional variable $\bm{w_{k,i}}$. In the forward message passing, there are four messages to be computed.

\begin{figure}[t]
  \centering
  \includegraphics[width=0.98\columnwidth]{./figures/Fig6.eps}\\
  \caption{The forward message passing from $\bm{W_{k,i}}$ to $\bm{W_{k+1,i}}$ (in blue) and the backward message passing from $\bm{W_{k+1,i}}$ to $\bm{W_{k,i}}$ (in green).}
\label{fig:6}
\end{figure}

1) The message passed from the bottom, denoted by $f_b(\bm{w_{k,i}})$. This message carries the information about $\bm{w_{k,i}}$ contained in the sample $y_{k,i}$. As per \eqref{eq:samples},
\begin{eqnarray*}
\hspace{-0.65cm} && y_{k,i}=\sum_{m=1}^M (h^\mathfrak{r}_{m}+jh^\mathfrak{i}_{m})(b^\mathfrak{r}_m+jb^\mathfrak{i}_m) + ({z}^\mathfrak{r}_{k,i}  + j{z}^\mathfrak{i}_{k,i}) \\
\hspace{-0.65cm} && =\!\! \sum_{m=1}^M (h^\mathfrak{r}_{m}b^\mathfrak{r}_m\!-\!h^\mathfrak{i}_{m}b^\mathfrak{i}_m)\!+\!{z}^\mathfrak{r}_{k,i} \!+\! j\sum_{m=1}^M(h^\mathfrak{r}_{m}b^\mathfrak{i}_m\!+\!h^\mathfrak{i}_{m}b^\mathfrak{r}_m)\!+\!j{z}^\mathfrak{i}_{k,i},
\end{eqnarray*}
where ${z}^\mathfrak{r}_{k,i}$, ${z}^\mathfrak{i}_{k,i}$ $\sim\mathcal{N}(0,\frac{N_0}{2d_k})$.
Thus, the likelihood function $f(y_{k,i}|\bm{w_{k,i}})$ is Gaussian, giving
\begin{eqnarray*}
f(y_{k,i}|&&\hspace{-0.65cm}\bm{w_{k,i}})\! \propto\! \exp\left\{\!\!-\frac{d_k}{N_0}\left[y^\mathfrak{r}_{k,i}\!-\!\!\sum_m (h^\mathfrak{r}_{m}b^\mathfrak{r}_m\!-\!h^\mathfrak{i}_{m}b^\mathfrak{i}_m)\right]^2 \!\right\} \\
&&\hspace{-0.6cm} \times \exp\left\{-\frac{d_k}{N_0}\left[y^\mathfrak{i}_{k,i}-\sum_m (h^\mathfrak{r}_{m}b^\mathfrak{i}_m+h^\mathfrak{i}_{m}b^\mathfrak{r}_m)\right]^2 \right\}.
\end{eqnarray*}

When we pass the information bottom up, $y_{k,i}$ is our observation (hence a constant) and $\bm{w_{k,i}}$ is the variable. Therefore, $f_b(\bm{w_{k,i}})=f(y_{k,i}|\bm{w_{k,i}})$.
After some manipulations, we can write $f_b(\bm{w_{k,i}})$ as a $2M$-dimensional Gaussian distribution:
\begin{eqnarray}\label{eq:fb}
f_b(\bm{w_{k,i}})\propto \mathcal{N}(\bm{w_{k,i}}, \bm{\eta_b}, \bm{\Sigma_b}),
\end{eqnarray}
where $\bm{\eta_b}$ and $\bm{\Sigma_b}$ are defined as
\begin{eqnarray}\label{eq:fb_params}
\bm{\eta_b} = \frac{2d_k}{N_0}
\begin{bmatrix}
\bm{\beta_1} \\
\bm{\beta_2}
\end{bmatrix}
\begin{bmatrix}
y^\mathfrak{r}_{k,i} \\
y^\mathfrak{i}_{k,i}
\end{bmatrix},~~
\bm{\Sigma_b} = \frac{2d_k}{N_0}
\begin{bmatrix}
\bm{\beta_1}\bm{\beta_1}^\top & \bm{\beta_1}\bm{\beta_2}^\top \\
\bm{\beta_2}\bm{\beta_1}^\top & \bm{\beta_1}\bm{\beta_1}^\top
\end{bmatrix},
\end{eqnarray}
and the matrices $\bm{\beta_1}$ and $\bm{\beta_2}$ are composed of channel coefficients as follows:
\begin{eqnarray*}
\bm{\beta_1}=
\begin{bmatrix}
h^\mathfrak{r}_{1} & h^\mathfrak{i}_{1} \\
h^\mathfrak{r}_{2} & h^\mathfrak{i}_{2} \\
\vdots & \vdots \\
h^\mathfrak{r}_{M} & h^\mathfrak{i}_{M} \\
\end{bmatrix},~~
\bm{\beta_2}=
\begin{bmatrix}
-h^\mathfrak{i}_{1} & h^\mathfrak{r}_{1} \\
-h^\mathfrak{i}_{2} & h^\mathfrak{r}_{2} \\
\vdots & \vdots \\
-h^\mathfrak{i}_{M} & h^\mathfrak{r}_{M} \\
\end{bmatrix}.
\end{eqnarray*}

In \eqref{eq:fb_params}, we have assumed that the dimensionality of $\bm{w_{k,i}}$ is $2M$, that is, $y_{k,i}=y_k[i]$ is related to $M$ complex variables. However, this is only valid when the number of neighbor symbols of $y_k[i]$ is $M$.
As shown in \eqref{eq:neighbors}, $\left|\mathcal{V}(y_k[i])\right|=M$ only when $1< i\leq L$. Thus, we can compute $\bm{\eta_b}$ and $\bm{\Sigma_b}$ by \eqref{eq:fb_params} only when $1< i\leq L$.

For the boundary samples ($i=1$, $L+1$) whose neighbor symbols are less than $M$, we further multiply the parameters $\bm{\eta_b}$ and $\bm{\Sigma_b}$ in \eqref{eq:fb_params} by an indicator vector $\bm{\gamma}$ and an indicator matrix $\bm{\Gamma}$, respectively, to ensure that $f_b(\bm{w_{k,i}})$ does not contain information about the symbols that do not belong to $\mathcal{V}(y_k[i])$. The general form of $\bm{\eta_b}$ and $\bm{\Sigma_b}$ are
\begin{eqnarray}\label{eq:fb_params2}
&& \bm{\eta_b} = \frac{2d_k}{N_0}
\begin{bmatrix}
\bm{\beta_1} \\
\bm{\beta_2}
\end{bmatrix}
\begin{bmatrix}
y^\mathfrak{r}_{k,i} \\
y^\mathfrak{i}_{k,i}
\end{bmatrix}\circ \bm{\gamma_k},  \\\label{eq:fb_params3}
&& \bm{\Sigma_b} = \frac{2d_k}{N_0}
\begin{bmatrix}
\bm{\beta_1}\bm{\beta_1}^\top & \bm{\beta_1}\bm{\beta_2}^\top \\
\bm{\beta_2}\bm{\beta_1}^\top & \bm{\beta_1}\bm{\beta_1}^\top
\end{bmatrix} \circ \bm{\Gamma_k},
\end{eqnarray}
where $\circ$ is an elementwise multiplication. The indicator vector $\bm{\gamma}$ and the indicator matrix $\bm{\Gamma}$ are defined as follows.

First, for the first $M$ samples (i.e., $i=1$), we have $\left|\mathcal{V}(y_k[i])\right|=k$ from \eqref{eq:neighbors}. Thus, we define
\begin{eqnarray*}
\bm{\gamma_k}=
\begin{bmatrix}
\begin{smallmatrix}
\bm{1}_{k\times 1} \\
\bm{0}_{(M\!-\!k)\times 1} \\
\bm{1}_{k\times 1} \\
\bm{0}_{(M\!-\!k)\times 1} \\
\end{smallmatrix}
\end{bmatrix},
\end{eqnarray*}
\begin{eqnarray*}
\bm{\Gamma_k}=
\begin{bmatrix}
\begin{smallmatrix}
\bm{1}_{k\times k}          &     \bm{0}_{k\times (M\!-\!k)}        &  \bm{1}_{k\times k}          &     \bm{0}_{k\times (M\!-\!k)}  \\
\bm{0}_{(M\!-\!k)\times k}   &      \bm{0}_{(M\!-\!k)\times (M\!-\!k)}   &      \bm{0}_{(M\!-\!k)\times k}   &      \bm{0}_{(M\!-\!k)\times (M\!-\!k)}   \\
\bm{1}_{k\times k}          &     \bm{0}_{k\times (M\!-\!k)}        &  \bm{1}_{k\times k}          &     \bm{0}_{k\times (M\!-\!k)}  \\
\bm{0}_{(M\!-\!k)\times k}   &      \bm{0}_{(M\!-\!k)\times (M\!-\!k)}   &      \bm{0}_{(M\!-\!k)\times k}   &      \bm{0}_{(M\!-\!k)\times (M\!-\!k)}
\end{smallmatrix}
\end{bmatrix},
\end{eqnarray*}
where $\bm{1}$ and $\bm{0}$ are all-ones and all-zero matrices with subscripts denoting their dimensions.

Second, for the last $M$ samples (i.e., $i=L+1$), we have $\left|\mathcal{V}(y_k[i])\right|=M-k$ from \eqref{eq:neighbors}. Thus, we define
\begin{eqnarray*}
\bm{\gamma_k}=
\begin{bmatrix}
\begin{smallmatrix}
\bm{0}_{k\times 1} \\
\bm{1}_{(M\!-\!k)\times 1} \\
\bm{0}_{k\times 1} \\
\bm{1}_{(M\!-\!k)\times 1} \\
\end{smallmatrix}
\end{bmatrix},
\end{eqnarray*}
\begin{eqnarray*}
\bm{\Gamma_k}=
\begin{bmatrix}
\begin{smallmatrix}
\bm{0}_{k\times k}          &     \bm{0}_{k\times (M\!-\!k)}        &  \bm{0}_{k\times k}          &     \bm{0}_{k\times (M\!-\!k)}  \\
\bm{0}_{(M\!-\!k)\times k}   &      \bm{1}_{(M\!-\!k)\times (M\!-\!k)}   &      \bm{0}_{(M\!-\!k)\times k}   &      \bm{1}_{(M\!-\!k)\times (M\!-\!k)}   \\
\bm{0}_{k\times k}          &     \bm{0}_{k\times (M\!-\!k)}        &  \bm{0}_{k\times k}          &     \bm{0}_{k\times (M\!-\!k)}  \\
\bm{0}_{(M\!-\!k)\times k}   &      \bm{1}_{(M\!-\!k)\times (M\!-\!k)}   &      \bm{0}_{(M\!-\!k)\times k}   &      \bm{1}_{(M\!-\!k)\times (M\!-\!k)}
\end{smallmatrix}
\end{bmatrix}.
\end{eqnarray*}

Finally, for all other samples ($1<i\leq L$), we simply set
\begin{eqnarray*}
\bm{\gamma_k}= \bm{1}_{2M\times 1},~~\bm{\Gamma_k}= \bm{1}_{2M\times 2M}.
\end{eqnarray*}
This is consistent with \eqref{eq:fb_params}.

2) Next, we consider the message $f_t(\bm{w_{k,i}})$ passed from the top. This message is the prior information of $\bm{w_{k,i}}$ and only added when $k=M$ (see Fig.~\ref{fig:5}). Therefore, we can write this message as
\begin{eqnarray*}
f_t(\bm{w_{k,i}})= \mathbbm{1}_{k=M}f_t(\bm{w_{M,i}}) + (1-\mathbbm{1}_{k=M})\bm{1}_{2M\times 1},
\end{eqnarray*}
that is, $f_t(\bm{w_{k,i}})$ is $f_t(\bm{w_{M,i}})$ when $k= M$ and an all-ones vector otherwise. In particular,
\begin{eqnarray}\label{eq:ft}
f_t(\bm{w_{M,i}})\propto \mathcal{N}(\bm{w_{M,i}}, \bm{\mu_t}, \bm{\Sigma_t}),
\end{eqnarray}
where
\begin{eqnarray*}
\hspace{-0.5cm}&& \bm{\mu_t}=\left[
\widehat{\mathbb{E}}_1^\mathfrak{r}, \widehat{\mathbb{E}}_2^\mathfrak{r}, ..., \widehat{\mathbb{E}}_M^\mathfrak{r},\widehat{\mathbb{E}}_1^\mathfrak{i}, \widehat{\mathbb{E}}_2^\mathfrak{i}, ..., \widehat{\mathbb{E}}_M^\mathfrak{i}\right]^\top,  \\
\hspace{-0.5cm}&& \bm{\Sigma_t} =
\frac{1}{2}\text{diag}\left(\widehat{\mathbb{D}}_1,\widehat{\mathbb{D}}_2,...,\widehat{\mathbb{D}}_M,\widehat{\mathbb{D}}_1,\widehat{\mathbb{D}}_2,...,\widehat{\mathbb{D}}_M\right).
\end{eqnarray*}
It is easy to transform the moment form of $f_t(\bm{w_{M,i}})$ to the canonical form by
\begin{eqnarray*}
f_t(\bm{w_{M,i}})\propto \mathcal{N}\left(\bm{w_{M,i}}; \bm{\eta_t} = \bm{\Sigma_t^\dagger \mu_t}, \bm{\Lambda_t=\Sigma_t^\dagger} \right).
\end{eqnarray*}

3) The third message, denoted by $f_\ell(\bm{w_{k,i}})$ in Fig.~\ref{fig:6}, is the message passed from $\bm{w_{k-1,i}}$ on the left. This message is obtained in the same way as $f_\ell(\bm{w_{k+1,i}})$ and we will analyze it at the end of forward message passing. For now, let us assume it is Gaussian and denote it by
\begin{eqnarray}\label{eq:fl}
f_\ell(\bm{w_{k,i}})\propto \mathcal{N}\left(\bm{w_{k,i}}; \bm{\eta_\ell}, \bm{\Lambda_\ell} \right).
\end{eqnarray}

4) As per the sum-product rule, the message out of a local function along an edge is the product of all incoming messages to this local function along all other edges. Thus, the message out of the equality function ``$=$'', denoted by $f_r(\bm{w_{k,i}})$ in Fig.~\ref{fig:6}, can be obtained by
\begin{eqnarray}
f_r(\bm{w_{k,i}})=f_b(\bm{w_{k,i}})f_t(\bm{w_{k,i}})f_\ell(\bm{w_{k,i}}).
\end{eqnarray}
This is the ``product'' step of the sum-product algorithm. From Lemma \ref{lemma2}, we know $f_r(\bm{w_{k,i}})$ is a Gaussian distribution, and
\begin{eqnarray}\label{eq:fr}
f_r(\bm{w_{k,i}})\propto \mathcal{N}\left(\bm{w_{k,i}}; \bm{\eta_r}, \bm{\Lambda_r} \right),
\end{eqnarray}
where $\bm{\eta_r}=\bm{\eta_b} +\bm{\eta_\ell}$, $\bm{\Lambda_r}=\bm{\Lambda_b}+ \bm{\Lambda_\ell}$. We emphasize that this message is an aggregation of all the known information about $\bm{w_{k,i}}$ from the left side of the graph.

The next step is to pass the message $f_r(\bm{w_{k,i}})$ through the compatibility function $\delta$. Notice that the compatibility function connects two different variables: on the LHS, the variable associated with the edge is $\bm{w_{k,i}}$; on the RHS, the variable associated with the edge is $\bm{w_{k+1,i}}$. Therefore, we have to integrate $f_r(\bm{w_{k,i}})$ over all variates that are in $\bm{w_{k,i}}$ but not in $\bm{w_{k+1,i}}$. This is the ``sum'' step of the sum-product algorithm.

Notice that the common variates of $\bm{w_{k,i}}$ and $\bm{w_{k+1,i}}$ are
\begin{eqnarray*}
\bm{w_\cap}=\left(b^\mathfrak{r}_1,...,b^\mathfrak{r}_k,b^\mathfrak{r}_{k+2},...,b^\mathfrak{r}_M,
b^\mathfrak{i}_1,...,b^\mathfrak{i}_k,b^\mathfrak{i}_{k+2},...,b^\mathfrak{i}_M \right),
\end{eqnarray*}
and the two different variates are $b^\mathfrak{r}_{k+1}$ and $b^\mathfrak{i}_{k+1}$ -- in $\bm{w_{k+1,i}}$, these two variates are $c^\mathfrak{r}_{k+1}$ and $c^\mathfrak{i}_{k+1}$.

Let us integrate $f_r(\bm{w_{k,i}})$ over $b^\mathfrak{r}_{k+1}$ and $b^\mathfrak{i}_{k+1}$, giving,
\begin{eqnarray*}
f(\bm{w_{\cap}})=\int_{b^\mathfrak{r}_{k+1}}\int_{b^\mathfrak{i}_{k+1}}f_r(\bm{w_{k,i}}) d b^\mathfrak{r}_{k+1} d b^\mathfrak{i}_{k+1}.
\end{eqnarray*}
As per Lemma \ref{lemma1}, $f(\bm{w_{\cap}})$ is also Gaussian. In particular, if we write $f_r(\bm{w_{k,i}})$ and $f(\bm{w_{\cap}})$ in moment form as
\begin{eqnarray*}
f_r(\bm{w_{k,i}}) \hspace{-0.2cm}& \propto &\hspace{-0.2cm} \mathcal{N}\left(\bm{w_{k,i}}; \bm{\mu_r}, \bm{\Sigma_r} \right), \\
f_r(\bm{w_{\cap}})\hspace{-0.2cm}& \propto &\hspace{-0.2cm} \mathcal{N}\left(\bm{w_{\cap}}; \bm{\mu_\cap}, \bm{\Sigma_\cap} \right),
\end{eqnarray*}
then $\bm{\mu_\cap}$ can be obtained by deleting the ($k+1$)-th and ($k+1+M$)-th rows of $\bm{\mu_r}$; $\bm{\Sigma_\cap}$ can be obtained by deleting the ($k+1$)-th and ($k+1+M$)-th rows and columns of $\bm{\Sigma_r}$.

However, $\bm{w_{\cap}}$ is a ($2M-2$) dimensional variable. To obtain $f_\ell(\bm{w_{k+1,i}})$, we have to expand the dimensionality of $\bm{w_{\cap}}$ by adding $c^\mathfrak{r}_{k+1}$ and $c^\mathfrak{i}_{k+1}$ in the ($k+1$)-th and ($k+1+M$)-th positions. After expansion, $f_\ell(\bm{w_{k+1,i}})$ is still multivariate Gaussian:
\begin{eqnarray}\label{eq:fl_right}
f_\ell(\bm{w_{k+1,i}})\propto \mathcal{N}\left(\bm{w_{k+1,i}}; \bm{\mu_\ell}, \bm{\Sigma_\ell} \right),
\end{eqnarray}
where $\bm{\mu_\ell}$ can be obtained by adding two zeros to $\bm{\mu_\cap}$; and $\bm{\Sigma_\ell}$ can be obtained by adding two all-zero rows and two all-zero columns to $\bm{\Sigma_\cap}$.

To summarize, we have shown that all the messages involved in the forward message passing are $2M$-dimensional multivariate Gaussians and can be parameterized by \eqref{eq:fb}, \eqref{eq:ft}, \eqref{eq:fl}, \eqref{eq:fr}, \eqref{eq:fl_right}, respectively.

{\it \textbf{Backward message passing}} -- Our tree structure is symmetric. Thus, backward message passing is symmetric to forward message passing. As shown in Fig.~\ref{fig:6}, to pass the messages from $\bm{w_{k+1,i}}$ and $\bm{w_{k,i}}$, we first compute three incoming messages $f_b(\bm{w_{k+1,i}})$, $f_t(\bm{w_{k+1,i}})$, and $f^\prime_r(\bm{w_{k+1,i}})$, where $f_b(\bm{w_{k+1,i}})$ and $f_t(\bm{w_{k+1,i}})$ are the same as that in the forward message passing and $f^\prime_r(\bm{w_{k+1,i}})$ is the message passed from $\bm{w_{k+2,i}}$ on the right.

Then, $f^\prime_\ell(\bm{w_{k+1,i}})$ and $f^\prime_r(\bm{w_{k,i}})$ are computed from ``product'' and ``sum'', respectively, by
\begin{eqnarray}
\label{eq:backward1}
f^\prime_\ell(\bm{w_{k+1,i}}) \hspace{-0.2cm} &=& \hspace{-0.2cm} f_b(\bm{w_{k+1,i}})f_t(\bm{w_{k+1,i}})f^\prime_r(\bm{w_{k+1,i}}), \\
\label{eq:backward2}
f^\prime_r(\bm{w_{k,i}})  \hspace{-0.2cm} &=&  \hspace{-0.2cm} \int_{c^\mathfrak{r}_{k+1}}\int_{c^\mathfrak{i}_{k+1}}f^\prime_\ell(\bm{w_{k,i}}) d c^\mathfrak{r}_{k+1} d c^\mathfrak{i}_{k+1}.
\end{eqnarray}

\begin{figure}[t]
  \centering
  \includegraphics[width=0.4\columnwidth]{./figures/Fig7.eps}\\
  \caption{The marginalization process in the sum-product algorithm.}
\label{fig:7}
\end{figure}

{\it \textbf{Marginalization}} -- After one forward message passing from left to right and one backward message passing from right to left, the marginal posterior distribution of each variable $\bm{w_{k,i}}$ converges and can be computed by
\begin{equation}\label{eq:mar}
{\displaystyle
f(\bm{w_{k,i}}|\bm{y}) \!=\! f_b(\bm{w_{k,i}})f_t(\bm{w_{k,i}})f_\ell(\bm{w_{k,i}})f^\prime_r(\bm{w_{k,i}}),}
\end{equation}
as illustrated in Fig.~\ref{fig:7}. Therefore, $f(\bm{w_{k,i}}\allowbreak|\allowbreak\bm{y})$ is a $2M$-dimensional real Gaussian distribution. In particular, if we write the four messages on the RHS of \eqref{eq:mar} in the canonical form, then the canonical parameters of $f(\bm{w_{k,i}}|\bm{y})$ is the sum of them.

Recall that
$\bm{w_{k,i}}=\allowbreak(b^\mathfrak{r}_1,\allowbreak ...,\allowbreak b^\mathfrak{r}_M,\allowbreak  b^\mathfrak{i}_1,...,\allowbreak b^\mathfrak{i}_M)$
is a $2M$ dimensional real random variable, where $b^\mathfrak{r}_m$ and $b^\mathfrak{i}_m$ are the real and imaginary parts of the $m$-th complex element of
$\bm{W_{k,i}}=\mathcal{V}(y_k[i])=(\allowbreak s_1[i],\allowbreak s_2[i],\allowbreak ...,\allowbreak s_k[i],\allowbreak s_{k+1}[i-1],\allowbreak s_{k+2}[i-1],...,\allowbreak s_M[i-1])$, thus, $f(\bm{W_{k,i}}|\bm{y})$ is an $M$-dimensional complex Gaussian distribution.

Let $k = M$, we have $\bm{W_{M,i}}=(s_1[i],s_2[i],...,s_M[i])=\bm{s[i]}$. This means
\begin{eqnarray}\label{eq:marginal}
f(\bm{s[i]}|\bm{y})=f(\bm{W_{k,i}}|\bm{y})
\end{eqnarray}
is an $M$-dimensional complex Gaussian, the mean and covariance of which can be computed from \eqref{eq:mar}.
